# Supplementary material for: Accurate Helium-Benzene Potential: from CCSD(T) to Gaussian Process Regression
Source: arXiv:2601.02166 source file (2026-01-05)
Supplement: Supplementary file 1 [file s0-main.tex]

\documentclass{article}

\input{../utils/preamble}

\title{
    \textbf{Supplementary Material for} \\[0.5cm]
    \Large Accurate Helium-Benzene Potential: from CCSD(T) to Gaussian Process Regression
}

\begin{document}

\maketitle

\pagebreak

\section{Molecular Geometries of Helium-Benzene Complex}

The benzene we used for this study has $R_{\text{CC}} = \SI{1.394}{\angstrom}$ and $R_{\text{CH}} = \SI{1.087}{\angstrom}$ respectively. Two different sets of He-benzene conformations were considered.  First, the helium atom was constrained to move on the $z$-axis only, with its $x$ and $y$ coordinates fixed. These molecular structures were used primarily for benchmarking purposes. A potential energy surface (PES) was generated using \ac{cc} calculations, and subsequently employed to benchmark the performance of various density functionals in describing the benzene-helium interaction. Fifty points were sampled along the $z$-axis for each functional and basis set combination under consideration. In the second set, a full three-dimensional PES was computed by placing the helium atom at 2475 different positions in the vicinity of the benzene molecule, spanning a range of $x$, $y$, and $z$ coordinates (Figure \ref{fig:3d_hebz_fig}). These calculations were performed using \ac{cc}, \ac{sapt}, and \ac{dft} methods. A reduced sampling strategy was employed, leveraging the symmetry of benzene. Calculations were performed within a $1/12$ slice of the $xy$ plane, with a radius of \SI{3}{\angstrom}, from the center of the benzene ring and a $z$-axis range of \SI{2.5}{\angstrom}, to \SI{7}{\angstrom}.

\begin{figure}[H]
    \centering
    \includegraphics[width=1\linewidth]{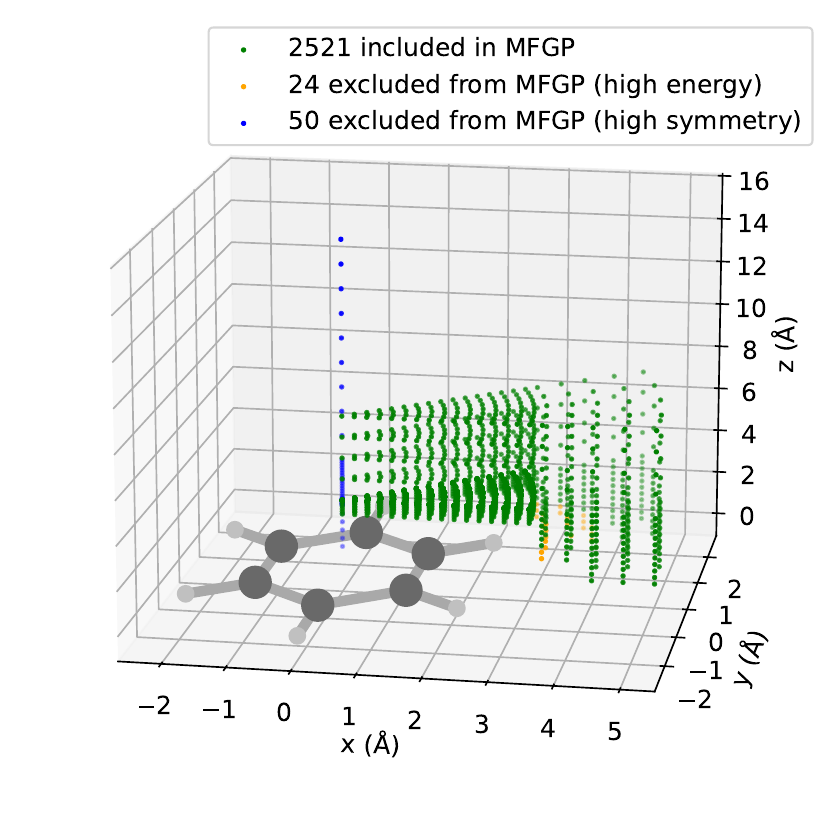}
    \caption{Helium-Benzene 2595 grid points denoting different positions of helium in the space computed with CCSD(T)/CBS. 2521 (green) positions were used to make a fit for MFGP.}
    \label{fig:3d_hebz_fig}
\end{figure}

\begin{figure}[H]
  \begin{subfigure}{\textwidth}
      \subcaption{}
    \centering\includegraphics[width=0.75\linewidth,height=\linewidth,keepaspectratio]{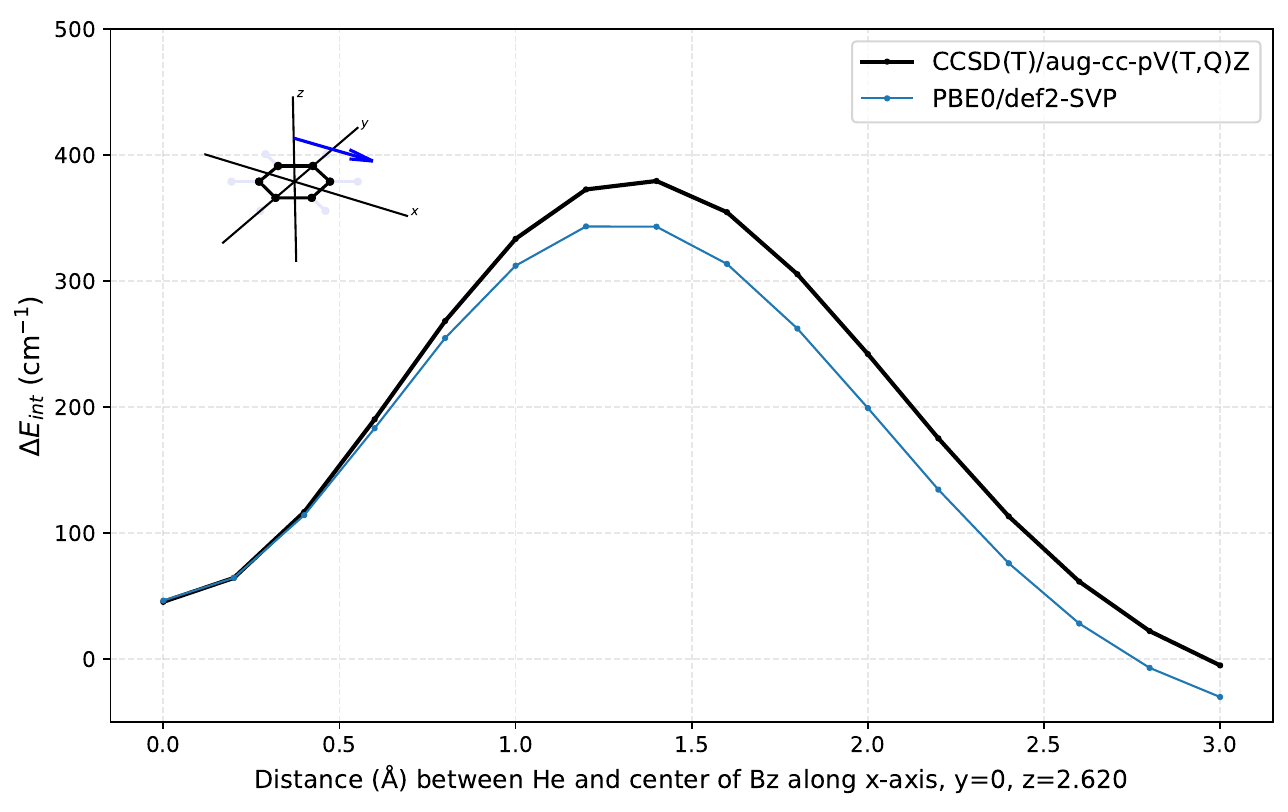}
  \end{subfigure}

  \begin{subfigure}{\textwidth}
        \subcaption{}

    \centering\includegraphics[width=0.75\linewidth,height=\linewidth,keepaspectratio]{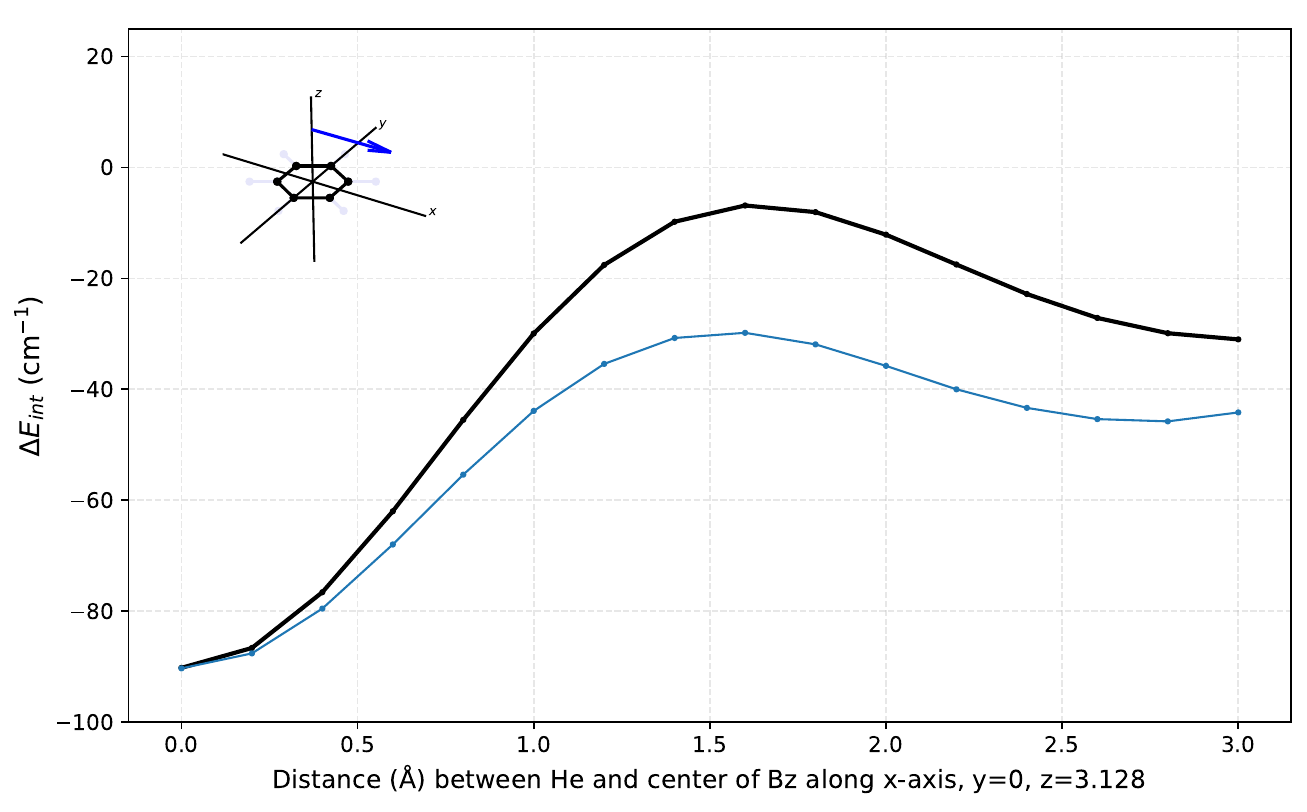}
  \end{subfigure}

  \begin{subfigure}{\textwidth}
        \subcaption{}

    \centering\includegraphics[width=0.75\linewidth,height=\linewidth,keepaspectratio]{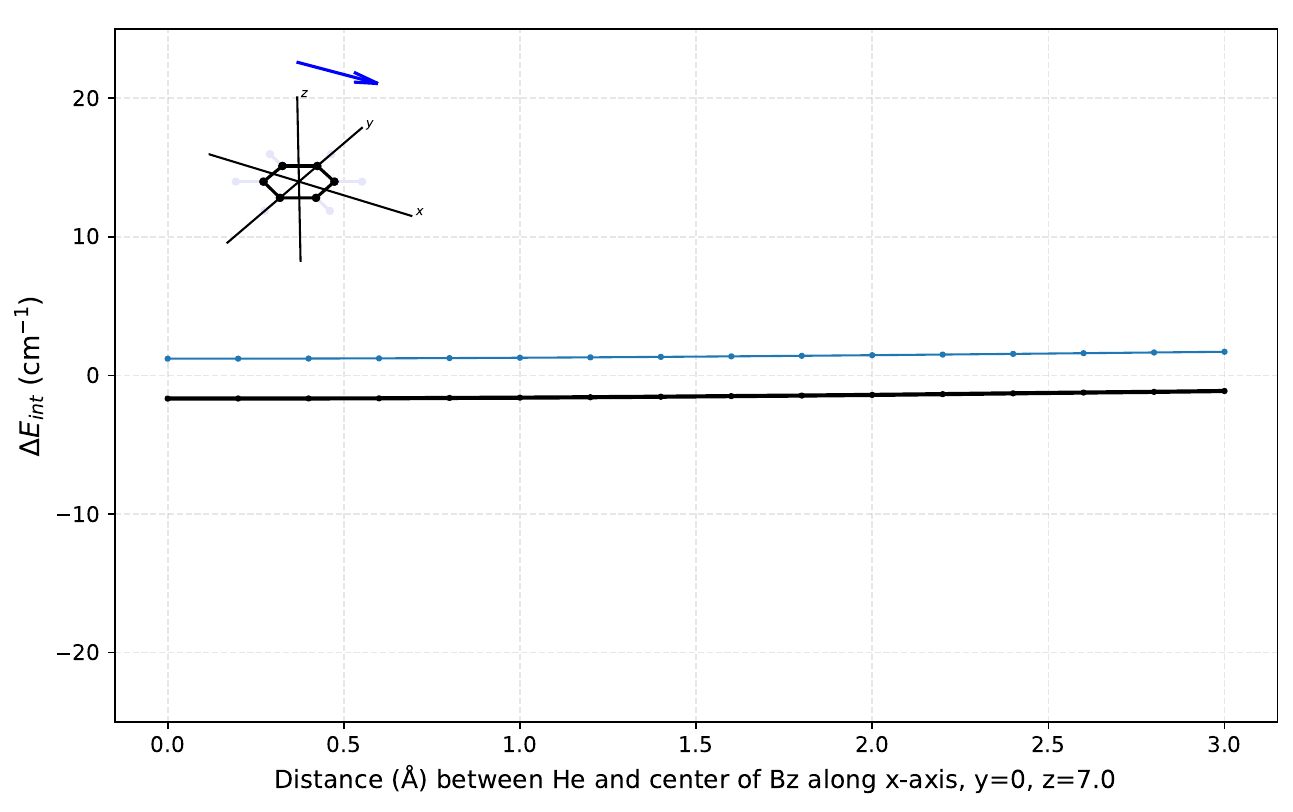}
  \end{subfigure}

\caption{PBE0 results}
\end{figure}\label{fig:dft_deviations}

\section{All DFT Functionals Benchmarking}

\begin{longtable}{lllccccc}

\toprule
\textbf{\#} & \textbf{Functionals} &   \textbf{Basis set} &        \textbf{MAE ($\si{\centi\meter^{-1}}$)}   &          \textbf{RMSE  ($\si{\centi\meter^{-1}}$)}&        \textbf{MAXE ($\si{\centi\meter^{-1}}$)} \\
\midrule
\endfirsthead

\toprule
\textbf{\#} & \textbf{Functionals} &   \textbf{Basis set} &        \textbf{MAE ($\si{\centi\meter^{-1}}$)}   &          \textbf{RMSE  ($\si{\centi\meter^{-1}}$)}&        \textbf{MAXE ($\si{\centi\meter^{-1}}$)} \\
\midrule

\endhead
\midrule

\endfoot

\bottomrule
\endlastfoot

 0 & pbe0      & def2-SVP    &  3.29e+00 &  3.35e+00 &  5.03e+00 \\
 1 & cam-b3lyp & def2-SVP    &  5.31e+00 &  6.37e+00 &  1.21e+01 \\
 2 & bh-lyp    & def2-TZVPP  &  7.96e+00 &  9.22e+00 &  1.67e+01 \\
 3 & bh-lyp    & def2-SVP    &  1.00e+01 &  1.09e+01 &  1.64e+01 \\
 4 & pbe       & def2-SVP    &  1.21e+01 &  1.22e+01 &  1.45e+01 \\
 5 & tpssh     & def2-TZVPP  &  1.26e+01 &  1.48e+01 &  2.74e+01 \\
 6 & bh-lyp    & def2-TZVPPD &  1.29e+01 &  1.43e+01 &  2.34e+01 \\
 7 & tpssh     & def2-SVP    &  1.37e+01 &  1.58e+01 &  2.96e+01 \\
 8 & tpss      & def2-SVP    &  1.39e+01 &  1.64e+01 &  3.17e+01 \\
 9 & tpss      & def2-TZVPP  &  1.42e+01 &  1.66e+01 &  3.03e+01 \\
10 & tpssh     & def2-SVPD   &  1.58e+01 &  1.78e+01 &  3.05e+01 \\
11 & bh-lyp    & def2-QZVPPD &  1.59e+01 &  1.76e+01 &  2.85e+01 \\
12 & bh-lyp    & def2-SVPD   &  1.60e+01 &  1.77e+01 &  2.81e+01 \\
13 & bh-lyp    & def2-QZVPP  &  1.69e+01 &  1.87e+01 &  3.05e+01 \\
14 & wb97x     & def2-SVP    &  1.70e+01 &  2.02e+01 &  3.56e+01 \\
15 & tpss      & def2-SVPD   &  1.89e+01 &  2.08e+01 &  3.44e+01 \\
16 & cam-b3lyp & def2-TZVPP  &  2.02e+01 &  2.24e+01 &  3.61e+01 \\
17 & tpssh     & def2-TZVPPD &  2.19e+01 &  2.42e+01 &  3.60e+01 \\
18 & tpssh     & def2-QZVPP  &  2.33e+01 &  2.49e+01 &  3.53e+01 \\
19 & tpss      & def2-TZVPPD &  2.61e+01 &  2.82e+01 &  4.09e+01 \\
20 & tpss      & def2-QZVPP  &  2.65e+01 &  2.81e+01 &  3.91e+01 \\
21 & cam-b3lyp & def2-TZVPPD &  2.71e+01 &  2.92e+01 &  4.37e+01 \\
22 & pbe0      & def2-TZVPP  &  2.75e+01 &  2.75e+01 &  2.93e+01 \\
23 & cam-b3lyp & def2-QZVPPD &  2.95e+01 &  3.18e+01 &  4.79e+01 \\
24 & cam-b3lyp & def2-QZVPP  &  3.02e+01 &  3.28e+01 &  5.00e+01 \\
25 & cam-b3lyp & def2-SVPD   &  3.52e+01 &  3.76e+01 &  5.61e+01 \\
26 & pbe0      & def2-SVPD   &  3.71e+01 &  3.74e+01 &  4.22e+01 \\
27 & pbe0      & def2-TZVPPD &  3.89e+01 &  3.90e+01 &  4.07e+01 \\
28 & pbe0      & def2-QZVPPD &  4.16e+01 &  4.17e+01 &  4.36e+01 \\
29 & pbe0      & def2-QZVPP  &  4.16e+01 &  4.18e+01 &  4.42e+01 \\
30 & pbe       & def2-TZVPP  &  4.51e+01 &  4.52e+01 &  4.72e+01 \\
31 & wb97x     & def2-QZVPP  &  5.02e+01 &  5.24e+01 &  6.94e+01 \\
32 & wb97x     & def2-TZVPP  &  5.02e+01 &  5.28e+01 &  7.14e+01 \\
33 & wb97x     & def2-QZVPPD &  5.15e+01 &  5.37e+01 &  7.10e+01 \\
34 & wb97x     & def2-TZVPPD &  5.29e+01 &  5.54e+01 &  7.36e+01 \\
35 & pbe       & def2-SVPD   &  5.90e+01 &  5.94e+01 &  6.52e+01 \\
36 & wb97x     & def2-SVPD   &  6.23e+01 &  6.71e+01 &  9.50e+01 \\
37 & pbe       & def2-TZVPPD &  6.30e+01 &  6.32e+01 &  6.63e+01 \\
38 & pbe       & def2-QZVPP  &  6.36e+01 &  6.40e+01 &  6.78e+01 \\
39 & m06       & def2-QZVPPD &  6.37e+01 &  6.53e+01 &  9.07e+01 \\
40 & pbe       & def2-QZVPPD &  6.61e+01 &  6.64e+01 &  6.99e+01 \\
41 & b2-plyp   & def2-QZVPP  &  7.01e+01 &  7.13e+01 &  9.15e+01 \\
42 & b2-plyp   & def2-QZVPPD &  7.03e+01 &  7.16e+01 &  9.27e+01 \\
43 & b2-plyp   & def2-SVPD   &  7.08e+01 &  7.25e+01 &  9.49e+01 \\
44 & b2-plyp   & def2-TZVPPD &  7.31e+01 &  7.45e+01 &  9.71e+01 \\
45 & m06-2x    & def2-QZVPPD &  7.38e+01 &  7.45e+01 &  8.93e+01 \\
46 & m06       & def2-QZVPP  &  7.49e+01 &  7.73e+01 &  1.04e+02 \\
47 & m06-2x    & def2-TZVPPD &  7.67e+01 &  7.73e+01 &  9.22e+01 \\
48 & m06-2x    & def2-TZVPP  &  7.68e+01 &  7.76e+01 &  9.38e+01 \\
49 & m06-2x    & def2-SVP    &  7.77e+01 &  8.00e+01 &  1.03e+02 \\
50 & b2-plyp   & def2-TZVPP  &  8.03e+01 &  8.18e+01 &  1.05e+02 \\
51 & m06       & def2-TZVPPD &  8.56e+01 &  8.76e+01 &  1.22e+02 \\
52 & b2-plyp   & def2-SVP    &  9.28e+01 &  9.48e+01 &  1.21e+02 \\
53 & m06       & def2-TZVPP  &  1.02e+02 &  1.05e+02 &  1.36e+02 \\
54 & pw6b95    & def2-SVP    &  1.09e+02 &  1.13e+02 &  1.57e+02 \\
55 & pw6b95    & def2-TZVPP  &  1.13e+02 &  1.16e+02 &  1.60e+02 \\
56 & m06-2x    & def2-SVPD   &  1.15e+02 &  1.18e+02 &  1.51e+02 \\
57 & pw6b95    & def2-TZVPPD &  1.18e+02 &  1.21e+02 &  1.67e+02 \\
58 & pw6b95    & def2-QZVPPD &  1.23e+02 &  1.27e+02 &  1.76e+02 \\
59 & pw6b95    & def2-QZVPP  &  1.29e+02 &  1.32e+02 &  1.80e+02 \\
60 & m06       & def2-SVP    &  1.37e+02 &  1.40e+02 &  1.76e+02 \\
61 & pw6b95    & def2-SVPD   &  1.45e+02 &  1.50e+02 &  1.90e+02 \\
62 & m06       & def2-SVPD   &  1.61e+02 &  1.63e+02 &  1.92e+02 \\
63 & b3lyp     & def2-SVPD   &  1.71e+02 &  1.75e+02 &  2.20e+02 \\
64 & blyp      & def2-SVPD   &  1.71e+02 &  1.75e+02 &  2.20e+02 \\
65 & b3lyp     & def2-TZVPPD &  1.76e+02 &  1.79e+02 &  2.29e+02 \\
66 & blyp      & def2-TZVPPD &  1.76e+02 &  1.79e+02 &  2.29e+02 \\
67 & blyp      & def2-QZVPPD &  1.77e+02 &  1.81e+02 &  2.30e+02 \\
68 & b3lyp     & def2-QZVPPD &  1.77e+02 &  1.81e+02 &  2.30e+02 \\
69 & b3lyp     & def2-QZVPP  &  1.80e+02 &  1.83e+02 &  2.31e+02 \\
70 & blyp      & def2-QZVPP  &  1.80e+02 &  1.83e+02 &  2.31e+02 \\
71 & b3lyp     & def2-TZVPP  &  1.85e+02 &  1.89e+02 &  2.40e+02 \\
72 & blyp      & def2-TZVPP  &  1.85e+02 &  1.89e+02 &  2.40e+02 \\
73 & blyp      & def2-SVP    &  2.05e+02 &  2.10e+02 &  2.64e+02 \\
74 & b3lyp     & def2-SVP    &  2.05e+02 &  2.10e+02 &  2.64e+02 \\
75 & tpssh     & def2-QZVPPD &  5.35e+04 &  2.67e+05 &  1.34e+06 \\
76 & m06-2x    & def2-QZVPP  &  8.70e+04 &  4.35e+05 &  2.17e+06 \\
77 & tpss      & def2-QZVPPD &  2.72e+05 &  1.36e+06 &  6.79e+06 \\

\caption{DFT benchmark analysis for the all functionals.}
\label{tab:dft_full_bench}
\end{longtable}

\section{Artifacts Arising From Joining Functions}
As pointed out in the main text, and seen in panel (c) of Figure 8, there is an unphysical dip in the potential along the cut $x=\SI{4.5}{\angstrom}, y=0, z=\SIrange{3}{4}{\angstrom}$ previously reported in Ref.~\cite{Shirkov_2024}. 
\begin{figure}[H]
    \centering
    \includegraphics[width=1\linewidth]{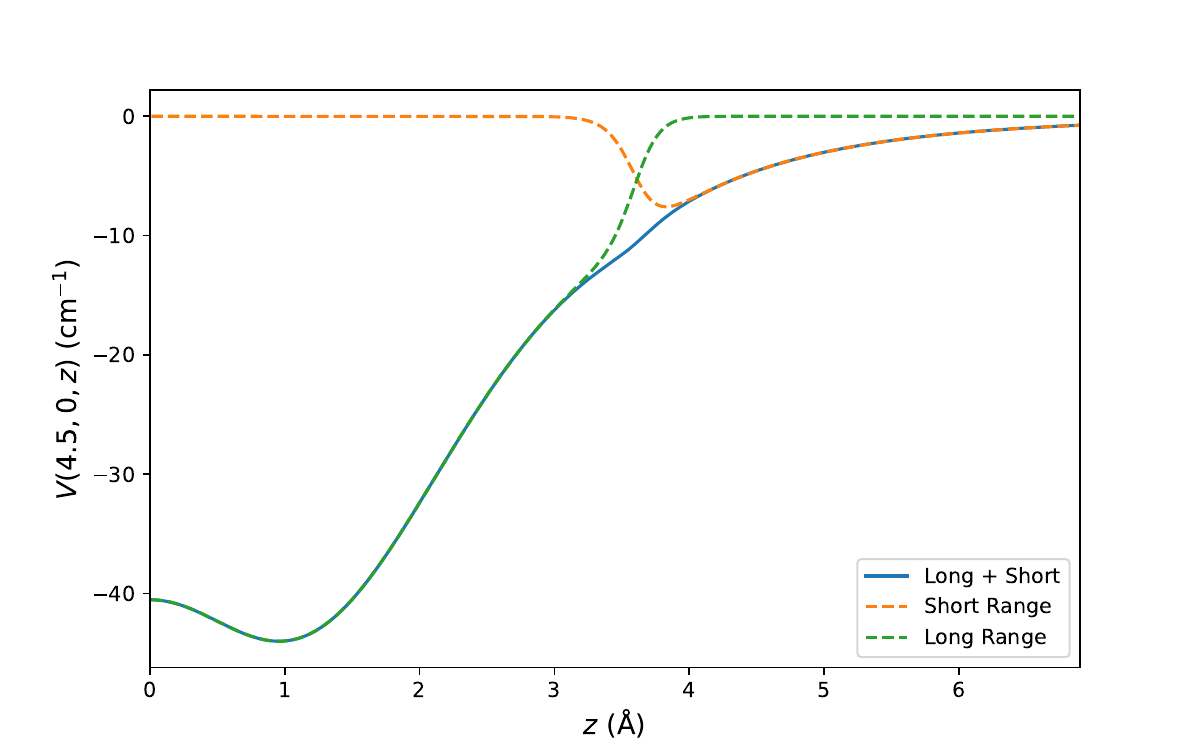}
    \caption{Illustration of the two different parts of the potential in \supercite{Shirkov_2024} and how the different damping functions introduce a unphysical dip in the PES. The dip occurs exactly at $z_0 = \sqrt{r_0^2 - 4.5^2 - 0^2}$ as expected.}
    \label{fig:Switching}
\end{figure}
The origin of this artifact the use of two different empirical functions to describe the short and long range parts of the potential which were glued  together via a damping functions. While this process ensures continuity of the potential, continuity of the derivative is not enforced as shown in \ref{fig:Switching}.  The dip occurs exactly at $r = r_0$ where the two functions crossover. One possible way to fix this would be the use a more complicated $C^2$ switching function. However our multifidelity approach offers a natural solution by ensuring the gaussian process potential has the correct long range physics in the switching regime from low-fidelity data. Thus, a simple switching function is enough to connect different scales. Since the physics at long distances is well understood, dense low fidelity data can always be generated to ensure the switching is smooth.
\printbibliography
\end{document}
